# Supplementary material for: A 3D measurement workflow for assessing replication quality and tool degradation in moulded microfluidic channels
Source: arXiv:2610.39046 source file (2026-10-28)
Supplement: Supplementary file 2 [file s2_numbers.tex]

\newcommand{\eqHT}{40}
\newcommand{\eqRTK}{52}
\newcommand{\eqW}{below the range}
